# Supplementary material for: Strategic Analysis of Griefing Attack in Lightning Network
Source: arXiv:2203.10533 source file (2022-12-20)
Supplement: Supplementary file 1 [file Appendix.pdf]

# Strategic Analysis and Countermeasure for Griefing Attack in Lightning Network

Subhra Mazumdar, Prabal Banerjee, Abhinandan Sinha, Sushmita Ruj, *Senior Member, IEEE,* and Bimal Kumar Roy

## SUPPLEMENTAL MATERIAL

### A. *Another form of Griefing Attack*

An attacking **B** waits and the rejects the payment at time $t' = D - \delta$, where $\delta \to 0$. **A** will not close the channel as **B** has responded before the timeout period elapses. We model interaction between **A** and **B** as a sequential *incomplete information game* $\Gamma_{HTLC-Penalty}$, shown in Fig. S1.

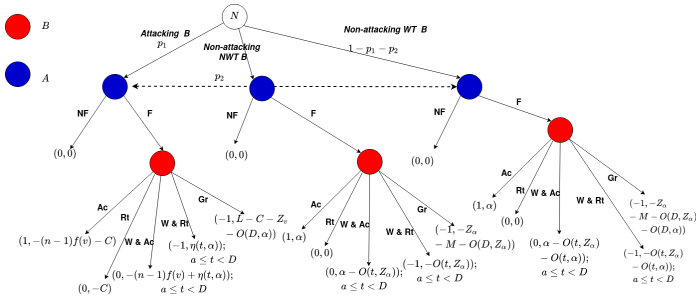


Fig. S1: Extensive form of the game $\Gamma_{HTLC-Penalty}$, when remuneration offered is $L$

*1) Game Model of HTLC with Penalty, remuneration offered is L:* The game begins with Nature (**N**) choosing the type of **B**, either *attacking* with probability $p_1$, *non-attacking, not willing to trade* with probability $p_2$ and *non-attacking, willing to trade* with probability $1-p_1-p_2$, respectively. When **A** gets a payment request to be forwarded to **B**, it decides either to *forward* ($F$) the payment or it can choose *not forward* ($NF$), remaining unaware of **B**'s type. If **A** had perfect knowledge regarding **B**'s type, then it would have selected *forward* in case of non-attacking **B** and remained idle in case of attacking **B**. If **A** has forwarded the payment, then **B** can choose its action from the following: *accept the payment* or *Ac*, *reject the payment* or *Rt*, *wait and then accept* or *W & Ac*, *wait and then reject* or *W & Rt*, and *grief* or *Gr*.

***Definition** 1:* The extensive-form game $\Gamma_{HTLC-Penalty}$, represented in Fig.S1, is defined as tuple $\Gamma_{HTLC-Penalty} = \langle N, \Theta_{\mathbf{B}}, (S_{\mathbf{A}}, S_{\mathbf{B}}), p_{\mathbf{A}}, (u_{\mathbf{A}}, u_{\mathbf{B}})\rangle$:

- The set of players $N$ ={**A**,**B**}
- The type of player **B** defined as $\Theta_{\mathbf{B}} =$ {Attacking(at), non-attacking willing to trade(nat-wt), non-attacking not willing to trade(nat-nwt)}
- The set of actions for player **A**, $S_{\mathbf{A}} = \{F, NF\}$
- The set of actions for player **B**, $S_{\mathbf{B}} =$ {Ac, Rt, W & Ac, W & Rt, Gr}
- Probability function $p_{\mathbf{A}}$ is a function from $\Theta_{\mathbf{A}}$ into $\Delta(\Theta_{\mathbf{B}})$, the set of probability distribution over $\Theta_{\mathbf{B}}$. Since we are not bothered about player $\mathbf{A}'s$ type, $p_{\mathbf{A}}$ specifies a probability distribution over the set $\Theta_{\mathbf{B}}$ representing what player **A** beliefs about the type of player **B**. Here $p_{\mathbf{A}}(Attacking) = \theta$, $p_{\mathbf{A}}(Non\ \ Attacking, \text{not willing to trade}) = \theta_2$ and $p_{\mathbf{A}}(Non\ \ Attacking, \text{willing to trade}) = 1 - \theta - \theta_2$.
- The payoff function $u_i : \Theta \times S \to \mathbb{R}$ for $i \in \{\mathbf{A}, \mathbf{B}\}$, where $\Theta = \Theta_{\mathbf{B}}$ and $S = S_{\mathbf{A}} \times S_{\mathbf{B}}$, is such that for any profile of actions and any profile of types $(\hat{\theta}, s) \in \Theta \times S$, specifies the payoff the player $i$ would get, if players actual type were all as in $\hat{\theta}$ and the players all chose their action as in $s$.

*Payoffs of **A** and **B**:* If **A** chooses not to forward, then either party receives a payoff 0 since no off-chain contract got established, i.e., $u_{\mathbf{A}}(\theta_b, NF, s_b) = u_{\mathbf{B}}(\theta_b, NF, s_b) = 0, \theta_b \in \Theta_{\mathbf{B}}$ and $s_b \in S_{\mathbf{B}}$.

If **A** chooses $F$, each case has been analyzed below:

- **B** chooses not to attack and not willing to trade. It locks an amount $Z_\alpha$ as guarantee for timeperiod $D$ against the amount $\alpha$ forwarded by **A**. We analyze each case based on **B**'s time taken to resolve payment.
  - Instantaneous Response, i.e., $0 \leq t < a$:
    - ***B** accepts the payment*: Its payoff is $\alpha$. **A** has successfully forwarded the amount, and later it can claim the processing fee from is predecessor, thus its payoff is 1.
    - ***B** rejects the payment*: Both **A** and **B**'s payoff is 0, as none of them gains anything, and the channel balance is restored.
  - Delayed Response, i.e., $a \leq t < D$:
    1) ***B** waits and then accepts the payment*: **A** has $\alpha$ coins locked in contract formed with **B** as well as amount $Z_{\alpha,n-1}$ remains locked with the preceding contract. Payoff of **A**, if **B** delays in accepting payment, is $1 - 1 = 0$.
    
       While forming an off-chain contract with **A**, **B** need not deposit any coins. But with the introduction of penalty, it has to lock $Z_\alpha$ for accepting a conditional payment of amount $\alpha$. Delaying leads to loss of profit it could have earned had it utilized $Z_\alpha$ for

Subhra Mazumdar and Prabal Banerjee are with Cryptology and Security Research Unit, Abhinandan Sinha is with Economic Research Unit and Bimal Kumar Roy is with Applied Statistics Unit, all the units are affiliated to Indian Statistical Institute Kolkata, India (e-mail: subhra.mazumdar1993@gmail.com, mail.prabal@gmail.com, link2abhinandan@gmail.com, bimal@isical.ac.in)

Prabal Banerjee is also with Polygon (previously Matic Network).

Sushmita Ruj is with CSIRO's Data61 & UNSW Sydney, Australia (e-mail: sushmita.ruj@data61.csiro.au)

timeperiod $t$, denoted as $O(t, Z_\alpha)$. Thus, payoff of **B** upon delayed acceptance, is defined as $\alpha - O(t, Z_\alpha)$,

2) ***B** waits and then rejects the payment*: The loss incurred is the same as the previous case, except that the payment doesn't succeed. Hence, the payoff of **A** is $-1$ and **B**'s payoff is $-O(t, Z_\alpha)$.

- ***B** griefs*: The payoff defined for this situation is same as **B** delays in rejecting a payment till timeperiod $D$. But griefing leads to penalization of **B** and the penalty deducted from **B**'s balance is used for compensating **A**. Thus 1 is added to **A**'s payoff to show the rise in satisfaction level on obtaining compensation, i.e., $-2+1=-1$. Delaying leads to loss of profit it could have earned had it utilized $Z_\alpha$ for timeperiod $D$, denoted as $O(D, Z_\alpha)$. Payoff of **B** is $-M - O(D, Z_\alpha) - Z_\alpha$.

- **B** chooses not to attack, but it is willing to trade. We analyze each case based on **B**'s time taken to resolve payment.
  - Instantaneous Response, i.e., $0 \leq t < a$: Upon instant acceptance or rejection of payment, the payoffs for both **A** and **B** is the same as that observed in previous case.
  - Delayed Response, i.e., $a \leq t < D$:

    1) ***B** waits and then accepts the payment*: **A**'s payoff is 0. **B** incurs an additional loss of $O(t, \alpha)$ as it delays in accepting the payment and hence, fails to utilize the coins for trading. Thus, payoff of **B** upon delayed acceptance, is defined as $\alpha - O(t, Z_\alpha) - O(t, \alpha)$,

    2) ***B** waits and then rejects the payment*: The loss incurred is the same as the previous case, except that the payment doesn't succeed. Hence, the payoff of **A** is $-1$ and **B**'s payoff is $-O(t, Z_\alpha) - O(t, \alpha)$.
  - ***B** griefs*: The payoff defined for this situation is same as **B** delays in rejecting a payment till timeperiod $D$. But griefing leads to penalization of **B** and the penalty deducted from **B**'s balance is used for compensating **A**. Thus 1 is added to **A**'s payoff to show the rise in satisfaction level on obtaining compensation, i.e., $-2+1=-1$. Delaying leads to loss of profit it could have earned had it utilized $Z_\alpha$ for timeperiod $D$, denoted as $O(D, Z_\alpha)$. Additionally, it loses the profit by not claiming the coins from **A** and using it for trading. Payoff of **B** is $-M - O(D, Z_\alpha) - O(D, \alpha) - Z_\alpha$.

- Attacking **B** executes a self-payment of amount $v$ and forwards $v + (n-1)f(v)$. It has to additionally locked $Z_v$ as guarantee against the payment forwarded by node **A**. The amount of bribe offered is $L$ and **B** rejects the payment at time $t' \approx D$. We analyze each case as follows:
  - Instantaneous Response, i.e., $0 \leq t < a$:

    1) ***B** accepts the payment*: **B** ends up losing $(n-1)f(v)$, as it needs to pay $(n-1)$ intermediaries. It had already incurred a cost $C$. The payoff is $-(n-1)f(v) - C$. **A** has successfully forwarded the amount, hence its payoff is 1.

    2) ***B** rejects the payment*: $\mathbf{A}'s$ payoff is 0 and **B**'s payoff is $-C$.
  - Delayed Response, i.e., $a \leq t < D$:

    1) ***B** waits and then accepts the payment*: **A**'s payoff is 0 because of unutilized coins lying in the channel. **B** fails to earn any profit if it delays for timeperiod $t < D - \delta$. If it resolves just at $t' = D - \delta$, the external agent pays $L$. We define a function $\eta : \mathbb{W} \to \mathbb{R}^+$, where $\eta(t)$ specifies the net profit received for keeping amount $\alpha$ unutilized till time $t$, where:

$$\eta(t) = \begin{cases} -C - O(t, \alpha), & a < t < D - \delta \\ L - C - O(D-\delta, \alpha), & \text{otherwise} \end{cases} \quad (1)$$

    Delaying till time $t < D - \delta$, will not result in any profit, **B** loses the setup cost and the revenue had it utilized $\alpha$ for $t$ units of time. If it delays till $D - \delta$, it gets paid for the work done. Upon accepting a self-payment, it ends up paying a processing fee $f(v)$ to $n-1$ intermediaries. Thus, the payoff of **B** is $-(n-1)f(v) + \eta(t)$.

    2) ***B** waits and then rejects the payment*: Payoff of **A** is $-1$. Payoff of **B** is $\eta(t)$.
  - ***B** griefs*: **B** successfully mounts the attack, it gets a remuneration $L$ from external agent but at the same time loses $Z_v$ in order to compensate **A** and $C + O(D, \alpha)$ as additional cost. The payoff of **B** is $L - Z_v - C - O(D, \alpha)$. **A** gets compensated, hence its payoff is $-2+1=-1$ .

*Equilibrium Analysis:* If **A** plays $F$, a *non-attacking* **B**, irrespective of being *NWT* or *WT*, will choose *Ac* as its best response since $u_{\mathbf{B}}(nat-nwt, F, Ac) \geq u_{\mathbf{B}}(nat-nwt, F, s')$, $\forall s' \in S_{\mathbf{B}}$ and $u_{\mathbf{B}}(nat-wt, F, Ac) \geq u_{\mathbf{B}}(nat-wt, F, s'), \forall s' \in S_{\mathbf{B}}$. The attacking **B** chooses to *W & Rt* at time $t' = D - \delta$ since $\beta(D-\delta) = L - C - O(D-\delta, \alpha) > \alpha + O(D-\delta, \alpha)$. If **B** griefs, it loses $Z_v$.

Here, we have $\mathbb{E}_{\mathbf{A}}(F) = p(-1) + (1-p)(1)$ and $\mathbb{E}_{\mathbf{A}}(NF) = 0$. Expected payoff for forwarding is greater than that of not forwarding if $\theta = p < 0.5$. Hence, **A** chooses *Forward* if $\theta = p < 0.5$ else it chooses *Not Forward*; attacking **B** chooses *W & Rt* at time $t' = D - \delta$; non-attacking *NWT* **B** chooses *Accept*; non-attacking *WT* **B** chooses *Accept*; is a PBNE.

### B. Alternate Strategy for mounting Griefing Attack

We have proven in Claim 3 that given a budget $\mathcal{B}_{EX}$, if attacking **B** agrees to wait and reject the payment at time $T'$ : $\nu \leq T' < D$ for a remuneration $K \leq \frac{T'L(1+\gamma\frac{nD}{2}+\gamma\Delta\frac{n(2n-1)}{6})}{D(1+\gamma nD+\gamma\frac{n(n-1)\Delta}{2})}$, then the amount of collateral locked when HTLC with penalty is used is at least as high as the amount of penalty locked when HTLC was used. We model interaction between **A** and **B** as a sequential *incomplete information game* $\Gamma_{HTLC-Penalty}$, shown in Fig. S2.

*1) Game Model of HTLC with Penalty, remuneration offered is $K$:* The model is same as the one described in Section -A1. We define the payoff for each situation.

*Payoffs of **A** and **B**:* If **A** chooses not to forward, then either party receives a payoff 0 since no off-chain contract got established, i.e., $u_{\mathbf{A}}(\theta_b, NF, s_b) = u_{\mathbf{B}}(\theta_b, NF, s_b) = 0, \theta_b \in \Theta_{\mathbf{B}}$ and $s_b \in S_{\mathbf{B}}$.

If **A** chooses $F$, each case has been analyzed below:

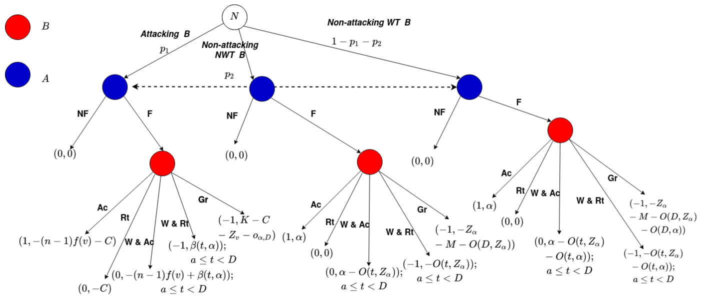


Fig. S2: Extensive form of the game $\Gamma_{HTLC-Penalty}$, when remuneration offered is $K$

- **B** chooses not to attack and not willing to trade, or it is willing to trade, the payoff for each case is the same as the payoff discussed for the game in Section -A1.
- Attacking **B** executes a self-payment of amount $v$ and forwards $v + (n-1)f(v)$. It has to additionally locked $Z_v$ as guarantee against the payment forwarded by node **A**. The amount of bribe offered is $K$ where $K < L$. **B** agrees to wait and then accept or reject the payment at time $T'$. Thus, it can be also stated that $K \approx \alpha + C + I(T', \alpha)$, where $I(T', \alpha)$ is the remuneration demanded for keeping $\alpha$ locked for $D$ units of time, $I(T', \alpha) > 2O(T', \alpha)$. We analyze each case as follows:
  - Instantaneous Response, i.e., $0 \le t < a$: The payoff is same as the one discussed in Section -A1.
  - Delayed Response, i.e., $a \le t < D$:
    1) ***B** waits and then accepts the payment*: **A**'s payoff is $0$ because of unutilized coins lying in the channel. **B** fails to earn any profit if it delays for timeperiod $t < T'$. If it resolves just at or after time $T'$, the external agent pays $K$. We define a function $\beta : \mathbb{W} \to \mathbb{R}^+$, where $\beta(t)$ specifies the net profit received for keeping amount $\alpha$ unutilized till time $t$, where:
    $$\beta(t) = \begin{cases} -C - O(t, \alpha), & a < t < T' \\ K - C - O(t, \alpha), & \text{otherwise} \end{cases} \tag{2}$$
    The payoff of **B** is $-(n-1)f(v) + \beta(t)$.
    2) ***B** waits and then rejects the payment*: Payoff of **A** is $-1$. Payoff of **B** is $\beta(t)$.
  - ***B** griefs*: **B** successfully mounts the attack, it gets a remuneration $K$ from external agent but at the same time loses $Z_v$ in order to compensate **A** and $C + O(D, \alpha)$ as additional cost. The payoff of **B** is $K - Z_v - C - O(D, \alpha)$. **A** gets compensated, hence its payoff is $-2 + 1 = -1$ .

*Equilibrium Analysis:* If **A** plays *F*, a *non-attacking* **B** will choose *Ac* as its best response since $u_{\mathbf{B}}(nat - nwt, F, Ac) \ge u_{\mathbf{B}}(nat - nwt, F, s'), \forall s' \in S_{\mathbf{B}}$ and $u_{\mathbf{B}}(nat - wt, F, Ac) \ge u_{\mathbf{B}}(nat - wt, F, s'), \forall s' \in S_{\mathbf{B}}$. The attacking **B** chooses to *W & Rt* at time $t = T'$ since $\beta(T') = K - C - O(T', \alpha) > \alpha + O(T', \alpha)$. If it delays beyond time $T'$, $\beta(t) = K - C - O(t, \alpha) > \alpha + O(T', \alpha) - O(t - T', \alpha)$, for $t > T'$.

Here, we have $\mathbb{E}_{\mathbf{A}}(F) = p(-1) + (1-p)(1)$ and $\mathbb{E}_{\mathbf{A}}(NF) = 0$. Expected payoff for forwarding is greater than that of not forwarding if $\theta = p < 0.5$. Hence, **A** chooses *Forward* if $\theta = p < 0.5$ else it chooses *Not Forward*; attacking **B** chooses *W & Rt* at time $t = T'$; non-attacking *NWT* **B** chooses *Accept*; non-attacking *WT* **B** chooses *Accept*; is a PBNE.
